# Supplementary material for: SharpNet: Fast and Accurate Recovery of Occluding Contours in Monocular Depth Estimation
Source: arXiv:1905.08598 source file (2019-11-11)
Supplement: Supplementary file 1 [file supplementary_materials.tex]

%%% To put in supplementary materials

\begin{table*}
	\begin{center}
		\begin{tabular}{|l||ll|ll|lll|}
			\hline
			Method & $\epsilon_{PE}^{plan} (cm) \downarrow$    & 
			$\epsilon_{PE}^{orie} (\deg) \downarrow$ & 
			$\epsilon_{DBE}^{acc} 
			(px) \downarrow$    & $\epsilon_{DBE}^{comp} (px) 
			\downarrow $ & 
			$\epsilon_{DDE}^{0} \uparrow$ & $\epsilon_{DDE}^{-} 
			\downarrow $ & 
			$\epsilon_{DDE}^{+} \downarrow $\\ \hline\hline
			Eigen \cite{Eigen14} & 6.65 & 25.62 & 5.48 & 70.31 & 72.06 
			& 25.71 
			& 2.23 \\
			Eigen \cite{Eigen2015PredictingDS} (AlexNet) & 6.34 & 21.74 
			& 4.57 
			& 46.52 & 78.24 & 17.86 & 3.90 \\
			Eigen \cite{Eigen2015PredictingDS} (VGG) & 4.93 & 17.18 & 
			4.51 & 
			43.64 & 80.73 & 17.47 & 1.80 \\
			Laina \cite{Laina2016DeeperDP} & 5.71 & 18.49 & 6.89 & 
			40.48 & 
			81.65 & 15.91 & 2.43 \\
			Liu \cite{LiuPAMI15} & 6.82 & 29.22 & 3.57 & 31.75 & 80.46 
			& 13.26 
			& 6.28 \\
			Li \cite{LiICCV17} & 6.22 & 20.17 & 3.68 & 36.27 & 84.13 & 
			12.49 & 
			3.38 \\
			Ours & 8.21 & 21.00 & \textbf{2.31} & 58.26 & 
			\textbf{85.95} & 
			\textbf{6.49}  & 7.56 \\ \hline
		\end{tabular}
	\end{center}
	\caption{Evaluation on metrics proposed by 
	\cite{Koch2018EvaluationOC} on 
	their dataset iBims-v1}
\end{table*}

\paragraph{Comparison with the iBims-v1 benchmark.}

\begin{table}[t]
	\begin{center}
		\resizebox{\linewidth}{!}{
			\begin{tabular}{|l|lll|lll|}
				\hline
				Method          & rel  & log  & rmse  & $\delta_1$ & $\delta_2$ 
& $\delta_3$ \\ \hline\hline
				Eigen           & 0.32 & 0.17 & 1.55  & 0.36   & 0.65   & 
0.84   \\ 
				Eigen (AlexNet) & 0.30 & 0.15 & 1.38  & 0.40   & 0.73   & 
0.88   \\ 
				Eigen (VGG)     & 0.25 & 0.13 & 1.26  & 0.47   & 0.78   & 
0.93   \\ 
				Laina           & 0.25 & 0.13 & 1.20  & 0.50   & 0.78   & 
0.91   \\ 
				Liu             & 0.30 & 0.13 & 1.26  & 0.48   & 0.78   & 
0.91   \\ 
				Li              & \textbf{0.22} & 0.11 & 1.07  & 0.59   & 
0.85   & 0.95   \\ 
				Ours            & 0.26 & \textbf{0.10} & \textbf{0.952} & 
\textbf{0.63} &  \textbf{0.87}   & 0.94   \\ \hline
		\end{tabular}}
	\end{center}
	\caption{Evaluation on depth estimation on the iBims-v1 dataset (our method 
was trained on \cite{Zhang2016pbrs} dataset then finetuned on NYUv2, while 
others were trained on NYUv2 only}
\end{table}

\paragraph{Comparison for scene reconstruction}

\begin{figure*}[t]
	\begin{center}
		\includegraphics[width=\linewidth]{augmentation_new2.pdf}
	\end{center}
	\caption{We present some augmentation on images and display the ability of 
	our method to retrieve sharp and accurate occlusion boundaries on depth 
	maps, making it suitable for augmented reality}
	\label{fig:augmentation}
\end{figure*}
